# Supplementary material for: 3D Occupancy Prediction with Low-Resolution Queries via Prototype-aware View Transformation
Source: arXiv:2503.15185 source file (2025-03-19)
Supplement: Supplementary file 1 [file X_suppl.tex]

\clearpage

\setcounter{page}{1}
\maketitlesupplementary

% \startcontents[section]
% \printcontents[section]{l}{1}{\setcounter{tocdepth}{2}}
\setcounter{section}{0}

\setcounter{table}{0}
\setcounter{figure}{0}

\section{Dataset Details}
\label{app:A}
In this section, we provide further details of the evaluation datasets Occ3D-nuScenes~\cite{tian2024occ3d} and SemanticKITTI~\cite{behley2019semantickitti}. 
Occ3D-nuScenes offers six surrounding multi-view camera images and a densely labeled semantic occupancy ground truth in the size of $200\times 200\times 16$. Each voxel represents one of 17 class labels in the $0.4m \times 0.4m \times 0.4m$ sized space of the real world. 700 and 150 scenes are used for training and validation, respectively. SemanticKITTI provides 22 outdoor driving scenarios, which includes 10 scenarios for training, 1 for validation, and 11 for testing. The ground truth scenes are voxelized in the dimension of $256\times 256\times 32$. Each voxel are in the size of $0.2m \times 0.2m \times 0.2m$ and are assigned with one of 20 classes~(19 semantic and 1 free space). To facilitate a broad understanding, we provide the configurations of Occ3D-nuScenes and SemanticKITTI datasets in the table below (see Table~\ref{tab:app_dataset}).

\begin{table}[h!]
    \centering
    \caption{Comparison of dataset configurations.}
    \resizebox{1.0\linewidth}{!}{
    \begin{tabular}{lcccc}
        \toprule
         Dataset & Output Res. & Voxel Size & \# Classes & \# Images \\
        \midrule
        Occ3d-nuScenes & $200\times 200\times 16$ & $0.4m \times 0.4m \times 0.4m$ & 12 & Multi-view \\
        SemanticKITTI & $256\times 256\times 32$ & $0.2m \times 0.2m \times 0.2m$ & 20 & Single \\        
        \bottomrule
     \end{tabular}}
     % \vspace{-0.3em}
    \label{tab:app_dataset}
\end{table}

\section{Experimental Details}
\label{app:B}
\subsection{Implementation Details}
\label{sec:B1}

\myparagraph{Occ3D-nuScenes.} 
 
We fix the weights for the occupancy loss and Lovasz loss as $\lambda_{1}=10.0$ and $\lambda_{2}=1.0$, respectively. Then we search the best-performing values of $\lambda_{3}$ and $\lambda_{4}$ within $\{1.0, 0.1, 0.01\}$, where we empirically find the optimal combination of $\lambda_{3}=0.1$ and $\lambda_{4}=0.01$ for \texttt{Tiny}, and $\lambda_{3}=1.0$ and $\lambda_{4}=1.0$ for \texttt{Small} and \texttt{Base}. Similarly, we search the values of $\tau_{\text{cls}}$ and $\tau_{\text{cons}}$ in between $\{0.3, 0.5\}$ and find that $\tau_{\text{cls}}=0.3$ and $\tau_{\text{cons}}=0.5$ produces the best result in the \texttt{Tiny} setting, and $\tau_{\text{cls}}=0.3$ and $\tau_{\text{cons}}=0.3$ for the \texttt{Small} and \texttt{Base} setting. 
All models are trained with 4 NVIDIA A100 GPUs.
The experiment configurations of Occ3D-nuScenes are summarized in Table~\ref{tab:config}.

\begin{table}[!htb]
    \centering
    \caption{Experimental Configurations of Occ3D-nuScenes.}
    \resizebox{\linewidth}{!}{%
    \begin{tabular}{llccc}
    \toprule
        & Specification  & \cellcolor{gray!15}\texttt{Tiny} & \cellcolor{gray!15}\texttt{Small} &
       \cellcolor{gray!15}\texttt{Base} \\
       \midrule
      \multirow{7}{*}{\rotatebox{90}{Model}} & Image resolution & $432\times800$ & $432\times800$ & $432\times800$ \\
                              & Image backbone & ResNet-101 & ResNet-101 & ResNet-101 \\
                              & FPN level & 5 & 5 & 5  \\
                              & Channel & 256 & 256 & 256  \\
                              & Encoder layer & 3 & 3 & 3  \\
                              & Decoder layer & 2 & 2 & 2   \\
                              & Query size & \cellcolor{yellow!7}$50\times50\times4$ & \cellcolor{yellow!7}$50\times50\times16$ & \cellcolor{yellow!7}$100\times100\times16$ \\
       \midrule
      
        \multirow{5}{*}{\rotatebox{90}{Training}} & Optimizer & AdamW & AdamW & AdamW  \\
        & Learning rate & 2e-4 & 2e-4 & 2e-4  \\
        & Scheduler & Cosine Annealing & Cosine Annealing & Cosine Annealing \\
        & Weight decay & 0.01 & 0.01 & 0.01  \\
        & Epoch & 12 & 12 & 12 \\
    \bottomrule
    \end{tabular}}
    \label{tab:config}
\end{table}

\myparagraph{SemanticKITTI.} 
For this task, we integrate our proposed strategies into two baseline models, VoxFormer~\cite{li2023voxformer} and Symphonies~\cite{jiang2024symphonize}.
We empirically determine the optimal hyperparameters of \{$\lambda_{3}$, $\lambda_{4}$, $\tau_{\text{cls}}$, $\tau_{\text{cons}}$\}: $\{1.0, 1.0, 0.3, 0.3\}$ for VoxFormer-\texttt{Small}, $\{1.0, 1.0, 0.5, 0.3\}$ for VoxFormer-\texttt{Base}, $\{1.0, 1.0, 0.3, 0.3\}$ for Symphonies-\texttt{Small} and $\{1.0, 1.0, 0.3, 0.5\}$ for Symphonies-\texttt{Base}. Similar to Occ3D-nuScenes, the models are trained with 4 NVIDIA A100 GPUs. The experimental configurations are summarized in Table~\ref{tab:config_semantickitti}.

\begin{table}[!htb]
    \centering
    \caption{Experimental Configurations on SemanticKITTI.}
    \resizebox{\linewidth}{!}{%
    \begin{tabular}{llcc|cc}
    \toprule
     & & \multicolumn{2}{c}{VoxFormer} & \multicolumn{2}{c}{Symphonies} \\
        & Specification  & \cellcolor{gray!15}\texttt{Small} & \cellcolor{gray!15}\texttt{Base} &
       \cellcolor{gray!15}\texttt{Small} & \cellcolor{gray!15}\texttt{Base} \\
       \midrule
      \multirow{7}{*}{\rotatebox{90}{Model}} & Image resolution & $370\times1200$ & $370\times1200$ & $370\times1206$ & $370\times1206$  \\
                              & Image backbone & ResNet-50 & ResNet-50 & ResNet-50 & ResNet-50 \\
                              & FPN level & 5 & 5 & 3 & 3  \\
                              & Channel & 128 & 128 & 128 & 128 \\
                              & Encoder layer & 3 & 3 & 1 & 1  \\
                              & Decoder layer & - & - & 3 & 3   \\
                              & Query size & \cellcolor{yellow!7}$64\times64\times8$ & \cellcolor{yellow!7}$128\times128\times16$ & \cellcolor{yellow!7}$64\times64\times8$ & \cellcolor{yellow!7}$128\times128\times16$ \\
       \midrule
       
        \multirow{5}{*}{\rotatebox{90}{Training}} & Optimizer & AdamW & AdamW & AdamW & AdamW  \\
        & Learning rate & 2e-4 & 2e-4 & 2e-4 & 2e-4  \\
        & Scheduler & Cosine Annealing & Cosine Annealing & MultiStep  & MultiStep \\
        & Weight decay & 0.01 & 0.01 & 0.0001 & 0.0001  \\
        & Epoch & 20 & 20 & 30 & 30 \\
    \bottomrule
    \end{tabular}}
    \label{tab:config_semantickitti}
\end{table}

\subsection{Baseline Details}
\label{app:BB}
In Table \textcolor{red}{1} of the main manuscript, we report the results of several strong baseline models: CTF-Occ~(NeurIPS'23)~\cite{tian2024occ3d}, BEVFormer~(ECCV'22)~\cite{li2022bevformer}, TPVFormer~(CVPR'23)~\cite{huang2023tri}, SurroundOcc~(ICCV'23)~\cite{wei2023surroundocc}, OccFormer~(ICCV'23)~\cite{zhang2023occformer} and PanoOcc~(CVPR'24)~\cite{wang2023panoocc}. However, since there are no official reports on the baseline results for \texttt{Small} and \texttt{Tiny} query settings, we select BEVFormer and PanoOcc as the main comparison targets and reproduce their results using the official code base. Also, since PanoOcc uses additional 3D object detection ground truth, we retrain the model without the detection loss for a fair comparison with our proposed ProtoOcc, which only trains with the occupancy ground truth. We additionally report the performance including the detection loss on PanoOcc in Table~\ref{tab:app_occ3d}. For SemanticKITTI, we additionally compare with MonoScene~(CVPR'22)~\cite{cao2022monoscene}, HASSC~(CVPR'24)~\cite{wang2024not}, VoxFormer~(CVPR'23)~\cite{li2023voxformer} and Symphonies~(CVPR'24)~\cite{jiang2024symphonize}. Here, we select VoxFormer and Symphonies as our main experimental baseline and plug our modules to observe their effectiveness.

% \begin{algorithm}[t!]
%   \caption{PyTorch Pseudo Code for Linear Mapping Function $\mathcal{H}$ in Eq.~\textcolor{red}{2}}
%   \label{alg:lin_map}
%   \begin{lstlisting}[style=pytorch]
% # Mapping affinity matrix A in 2D grid-cell (h’x w’).
% # N, M, K : number of view, number of prototype, number of hit query
% # h’, w’ :  spatial dimension
% # input:
% # A : affinity matrix, [N, M, K]
% # q_c: each query coordinate, [N, K, 1, 2]
% # output:
% # prototype_aware_pixel_feature: [N, M, h’, w’]
% def map_affinity_to_grid(A, q_c):
%     # get implicit 2D grid-cell
%     prototype_aware_pixel_feature = torch.zeros(N, M, |$h’$| * |$w’$|)
%     # get query coordinate
%     q_c = q_c[..., 0] * |$w’$|
%     q_c = q_c[..., 1] * |$h’$|
%     q_c = q_c.floor()
%     # filtering the value beyond the spatial shape
%     c_mask_x = torch.logical_and(q_c[..., 0] >= 0, q_c[..., 0] < |$w’$|)
%     c_mask_y = torch.logical_and(q_c[..., 1] >= 0, q_c[..., 1] < |$h’$|)
%     c_mask = torch.logical_and(c_mask_x, c_mask_y)
%     # get index and value
%     c_idx = q_c[..., 1] * |$w’$| + q_c[..., 0]
%     c_idx = (c_idx * c_mask).squeeze().unsqueeze(1).expand(N, M, -1)
%     c_val = A * c_mask.squeeze().unsqueeze(1).expand(N, M, -1)
%     # scatter similarity into the 2D grid-cell
%     prototype_aware_pixel_feature.scatter_add_(2, c_idx, c_val)
%     return prototype_aware_pixel_feature.reshape(N, M, |$h’$|, |$w’$|)
%   \end{lstlisting}
% \end{algorithm}

\begin{algorithm}[t!]
	\caption{PyTorch Pseudo Code for Linear Mapping Function $\mathcal{H}$ in Eq.\textcolor{red}{2}}
	\label{alg:lin_map}
	\begin{minted}
[
framesep=2mm,
baselinestretch=0.9,
fontsize=\footnotesize,
escapeinside=||,mathescape=true
]
{python}
# Mapping affinity matrix A in 2D grid-cell (h'x w').
# N, M, K, : number of view, number of prototype, number of hit query
# $\texttt{h}^\prime$, $\texttt{w}^\prime$:  spatial dimension

# input:
# A : affinity matrix, [N, M, K]
# q_c: each query coordinate, [N, K, 1, 2] 

# output: 
# prototype_aware_pixel_feature: [N, M, h', w']

def map_affinity_to_grid(A, q_c):
    # get implicit 2D grid-cell
    prototype_aware_pixel_feature = torch.zeros(N, M, |$\texttt{h}^\prime$|* |$\texttt{w}^\prime$|)
    
    # get query coordinate
    q_c = q_c[..., 0] * |$\texttt{w}^\prime$|
    q_c = q_c[..., 1] * |$\texttt{h}^\prime$|
    q_c = q_c.floor()
    
    # filtering the value beyond the spatial shape
    c_mask_x = torch.logical_and(q_c[..., 0] >= 0, q_c[..., 0] < |$\texttt{w}^\prime$|)
    c_mask_y = torch.logical_and(q_c[..., 1] >= 0, q_c[..., 1] < |$\texttt{h}^\prime$|)
    c_mask = torch.logical_and(c_mask_x, c_mask_y)
    
    # get index and value
    c_idx = q_c[..., 1] * |$\texttt{w}^\prime$| + q_c[..., 0]
    
    c_idx = (c_idx * c_mask).squeeze().unsqueeze(1).expand(N, M, -1)
    
    c_val = A * c_mask.squeeze().unsqueeze(1).expand(N, M, -1)
    
    # scatter similarity into the 2d gird-cell
    prototype_aware_pixel_feature.scatter_add_(2, c_idx, c_val)   

    return prototype_aware_pixel_feature.reshape(N, M, |$\texttt{h}^\prime$|, |$\texttt{w}^\prime$|)

\end{minted}
\end{algorithm}

\section{Method Details}
\label{app:C}
\subsection{Prototype-aware View Transformation}
\label{app:CA}
The core components of this process is prototype mapping and a contrastive learning based on pseudo ground truth masks.
To achieve prototype mapping, 2D prototype feature $\mathbf{P}_{\text{img}}$ should be first obtained from the given input images. 
We adopt the grouping technique of~\cite{ding2023hgformer} to generate $\mathbf{P}_{\text{img}}$, which is a widely used algorithm for clustering~\cite{achanta2012slic, jampani2018superpixel, yang2020superpixel}. Specifically, we set the downsampling ratio $r$ as 4, and the number of iterations for clustering as 6. 
Also, the contrastive learning with pseudo masks is necessary for enhancing the distinctiveness among the prototype features, thereby enriching the high-level contexts in voxel queries. 
In this stage, we develop a linear mapping function $\mathcal{H}$ for mapping 3D voxel prototype feature $\mathbf{P}_{\text{vox}}$ onto 2D grid-cell.
To enhance clarity and facilitate understanding, we provide a pseudo-code of linear mapping function $\mathcal{H}$ in Algorithm~\ref{alg:lin_map}. 
For this algorithm, we utilize an additional argument $\texttt{q}\_\texttt{c}$ indicating the coordinate of individual queries, which are obtained through the camera parameters during view transformation process.

\subsection{Multi-perspective Occupancy Decoding}
\label{app:CB}
Since feature-level voxel augmentations~(e.g., Random Dropout and Gaussian Noise) explicitly modify the feature values within the voxel queries, it is intuitive that they produce different contextual results when decoded. However, how do spatial-level voxel augmentations~(e.g., Transpose and Flips) create different contexts without any changes in the feature values? The answer to this question can be found in the shared-weight design of the transposed convolution network.

Consider a simple 2D case with $\begin{bmatrix}
a & b \\
c & d \\
\end{bmatrix}$ as the input and $\begin{bmatrix}
w & x \\
y & z \\
\end{bmatrix}$ as the kernel. Just as in the voxel queries, assume that each element of the input represents a specific region and is aware of its connectivity with the neighboring elements. Then, performing the 2D transposed convolution $\mathcal{C}_{2D}$ with strides as (1,1), we derive the following output:
\begin{multline*}
\label{eq:tc}
\mathcal{C}_{2D}^{(1,1)}\Big(
    \begin{bmatrix}
a & b \\
c & d \\
\end{bmatrix}, \begin{bmatrix}
w & x \\
y & z \\
\end{bmatrix}\Big)=\\\begin{bmatrix}
aw & ax + bw & bx\\
ay + c w& az + by + cx + dw & bz + dx\\
cy & cz + dy & dz\\
\end{bmatrix}.
\end{multline*}
The output elements are the linear combinations between the neighboring features, indicating a specific spatial context. Now we make spatial augmentations and apply $\mathcal{C}_{2D}$ with the same kernel. The result for the transposed input is formulated as:

\begin{multline*}
\mathcal{C}_{2D}^{(1,1)}\Big(
    \begin{bmatrix}
a & c \\
b & d \\
\end{bmatrix}, \begin{bmatrix}
w & x \\
y & z \\
\end{bmatrix}\Big)=\\\begin{bmatrix}
aw & ax + cw & cx\\
ay + bw& az + cy + bx + dw & cz + dx\\
by & bz + dy & dz\\
\end{bmatrix}.
\end{multline*}

\noindent Since the transposed input changes the spatial configuration of the original input, we re-do the spatial augmentation on the output to match the spatial locations between the augmentations:

\begin{multline*} 
\begin{bmatrix}
aw & ax + cw & cx\\
ay + bw& az + cy + bx + dw & cz + dx\\
by & bz + dy & dz\\
\end{bmatrix}\\\xRightarrow{\text{Re-do}}
\begin{bmatrix}
aw & ay + bw & by\\
ax + cw& az + cy + bx + dw & bz + dy\\
cx & cz + dx & dz\\
\end{bmatrix}.
\end{multline*}

\noindent Then, comparing this with the output from the first equation, we observe that each element, representing the feature of a specific region in the occupancy space, is made up of different linear combinations, indicating a distinct spatial context. For example, $ax+bw$ and $ay+bw$ in the identical position of each output indicates that they understand the context in that region uniquely by assigning different weights to features $a$ and $b$. Similarly, the 2D transposed convolution result of flipped input yields:

\begin{multline*}
\mathcal{C}_{2D}^{(1,1)}\Big(
    \begin{bmatrix}
d & c \\
b & a \\
\end{bmatrix}, \begin{bmatrix}
w & x \\
y & z \\
\end{bmatrix}\Big)=\\\begin{bmatrix}
dw & dx + cw & cx\\
dy + bw& dz + cy + bx + aw & cz + ax\\
by & bz + ay & az\\
\end{bmatrix},
\end{multline*}

\noindent and re-doing the same augmentation on the output produces:

\begin{multline*}   
\begin{bmatrix}
dw & cw+dx & cx\\
 bw+dy& aw +bx +cy+dz& ax+cz\\
by & ay+bz & az\\
\end{bmatrix}\\\xRightarrow{\text{Re-do}}
\begin{bmatrix}
az & ay+bz & by\\
ax + cz& aw +bx +cy+dz & bw + dy\\
cx & cw+dx & dw\\
\end{bmatrix}.
\end{multline*}
Note that we apply both horizontal and vertical flips for this augmentation. As a result, this creates another totally new context in each region. The same principle holds true for 3D transposed convolution used in our network. Therefore, we can conclude that the spatial augmentation with a transposed convolution is a valid strategy for contextual diversity.

\section{Additional Experimental Results}
\label{app:D}

\begin{table*}[t!]
		\scriptsize
		\setlength{\tabcolsep}{0.0050\linewidth}

		\centering
		\caption{\textbf{Comparison of the quantitative results on Occ3D-nuScenes~\cite{tian2024occ3d}.} $\dag$ demonstrates the variant of the \texttt{Base}, which utilizes the larger image resolution and more training duration. $\ddag$ utilizes external ground truth, particularly bounding boxes for 3D object detection.}
        \vspace{-0.2em}
            \scalebox{0.98}{
		\begin{tabular}{c|c| c | c c c c c c c c c c c c c c c c c}
			\toprule
			\shortstack{Query \\ Size} & \makecell{Model} & \makecell{mIoU}
                & \rotatebox{90}{\textcolor{others}{$\blacksquare$} others}
			& \rotatebox{90}{\textcolor{nbarrier}{$\blacksquare$} barrier}
			& \rotatebox{90}{\textcolor{nbicycle}{$\blacksquare$} bicycle}
			& \rotatebox{90}{\textcolor{nbus}{$\blacksquare$} bus}
			& \rotatebox{90}{\textcolor{ncar}{$\blacksquare$} car}
			& \rotatebox{90}{\textcolor{nconstruct}{$\blacksquare$} const. veh.}
			& \rotatebox{90}{\textcolor{nmotor}{$\blacksquare$} motorcycle}
			& \rotatebox{90}{\textcolor{npedestrian}{$\blacksquare$} pedestrian}
			& \rotatebox{90}{\textcolor{ntraffic}{$\blacksquare$} traffic cone}
			& \rotatebox{90}{\textcolor{ntrailer}{$\blacksquare$} trailer}
			& \rotatebox{90}{\textcolor{ntruck}{$\blacksquare$} truck}
			& \rotatebox{90}{\textcolor{ndriveable}{$\blacksquare$} drive. suf.}
			& \rotatebox{90}{\textcolor{nother}{$\blacksquare$} other flat}
			& \rotatebox{90}{\textcolor{nsidewalk}{$\blacksquare$} sidewalk}
			& \rotatebox{90}{\textcolor{nterrain}{$\blacksquare$} terrain}
			& \rotatebox{90}{\textcolor{nmanmade}{$\blacksquare$} manmade}
			& \rotatebox{90}{\textcolor{nvegetation}{$\blacksquare$} vegetation}
			\\
   
			\midrule

                \multirow{6}{*}{\shortstack{\texttt{Base}}}

                & BEVFormer~\cite{li2022bevformer} & \textcolor{lightgray}{34.97} & \textcolor{lightgray}{7.53} & \textcolor{lightgray}{41.77} & \textcolor{lightgray}{16.39} & \textcolor{lightgray}{44.06} & \textcolor{lightgray}{48.48} & \textcolor{lightgray}{17.27} & \textcolor{lightgray}{20.01} & 
                \textcolor{lightgray}{23.36} & \textcolor{lightgray}{21.16} & 
                \textcolor{lightgray}{28.88} & \textcolor{lightgray}{35.59} & \textcolor{lightgray}{80.12} & \textcolor{lightgray}{35.35} & 
                \textcolor{lightgray}{47.65} & \textcolor{lightgray}{51.89} & 
                \textcolor{lightgray}{40.68} & \textcolor{lightgray}{34.28} \\ %

                & PanoOcc~\cite{wang2023panoocc} & \textcolor{lightgray}{38.11} & \textcolor{lightgray}{9.75} & \textcolor{lightgray}{45.31} & \textcolor{lightgray}{22.45} & \textcolor{lightgray}{43.13} & \textcolor{lightgray}{50.19} & \textcolor{lightgray}{22.25} & \textcolor{lightgray}{27.35} & 
                \textcolor{lightgray}{24.49} & \textcolor{lightgray}{25.17} & 
                \textcolor{lightgray}{31.74} & \textcolor{lightgray}{37.95} & \textcolor{lightgray}{81.74} & \textcolor{lightgray}{42.29} & 
                \textcolor{lightgray}{50.82} & \textcolor{lightgray}{54.80} & 
                \textcolor{lightgray}{40.81} & \textcolor{lightgray}{37.14} \\ %

                & BEVFormer$^{\dagger}$ & \textcolor{lightgray}{38.91} & \textcolor{lightgray}{9.13} & \textcolor{lightgray}{48.22} & \textcolor{lightgray}{22.80} & \textcolor{lightgray}{47.30} & \textcolor{lightgray}{54.15} & \textcolor{lightgray}{21.86} & \textcolor{lightgray}{27.76} & \textcolor{lightgray}{27.48} & \textcolor{lightgray}{26.34} & \textcolor{lightgray}{32.69} & \textcolor{lightgray}{38.93} &  \textcolor{lightgray}{81.81} & \textcolor{lightgray}{39.89} & \textcolor{lightgray}{50.24} & \textcolor{lightgray}{53.03} & \textcolor{lightgray}{43.87} & \textcolor{lightgray}{35.97}  \\ %
                
                & PanoOcc$^{\dagger}$ & 41.33 & 11.60 & \textbf{50.74} & \textcolor{lightgray}{27.45} & \textbf{48.03} & \textcolor{lightgray}{53.50} & 23.41 & \textcolor{lightgray}{31.39} & 28.97 & \textcolor{lightgray}{29.07} & 34.78 & \textcolor{lightgray}{39.86} & \textcolor{lightgray}{83.10} & 45.44 & 54.00 & 56.63 & 44.53 & \textbf{40.08} \\ %

 & PanoOcc$^{\ddagger}$ & 41.60 & \textbf{11.99} & \textcolor{lightgray}{49.82} & 28.92 & \textcolor{lightgray}{45.46} & 54.78 & \textbf{25.2} & \textbf{32.93}
 & \textcolor{lightgray}{28.86} & \textbf{30.71} & \textcolor{lightgray}{33.87} & 41.32 & 83.18 & \textcolor{lightgray}{45.0} & \textcolor{lightgray}{53.80} & \textcolor{lightgray}{56.10} & \textcolor{lightgray}{45.11} & \textbf{40.1} \\ %
                
                & \cellcolor{gray!20} $\text{\textbf{ProtoOcc}}^{\dag}$~\textbf{(Ours)} &  \cellcolor{gray!20}\textbf{41.87} & \cellcolor{gray!20}\textcolor{lightgray}{11.47} & \cellcolor{gray!20}49.97 & \cellcolor{gray!20}\textbf{29.91} & \cellcolor{gray!20}47.75 & \cellcolor{gray!20}\textbf{55.07} & \cellcolor{gray!20}\textcolor{lightgray}{23.08} & \cellcolor{gray!20}32.22& \cellcolor{gray!20}\textbf{29.07} & \cellcolor{gray!20}29.38 & \cellcolor{gray!20}\textbf{35.17} & \cellcolor{gray!20}\textbf{42.02} & \cellcolor{gray!20}\textbf{83.66}& \cellcolor{gray!20}\textbf{45.82} & \cellcolor{gray!20}\textbf{54.7} & \cellcolor{gray!20}\textbf{57.51} & \cellcolor{gray!20}\textbf{44.95} & \cellcolor{gray!20}\textcolor{lightgray}{40.04}  \\ %

                \midrule

                \multirow{4}{*}{\shortstack{\texttt{Small}}}& BEVFormer~\cite{li2022bevformer} & \textcolor{lightgray}{33.98} & \textcolor{lightgray}{6.75} & \textcolor{lightgray}{41.67} & \textcolor{lightgray}{13.91} & \textcolor{lightgray}{41.97} & \textcolor{lightgray}{48.49} & \textcolor{lightgray}{17.83} & \textcolor{lightgray}{18.01} & \textcolor{lightgray}{22.19} & \textcolor{lightgray}{19.08} & \textcolor{lightgray}{29.64} & \textcolor{lightgray}{33.23} & \textcolor{lightgray}{79.42} & \textcolor{lightgray}{36.48} & \textcolor{lightgray}{46.82} & \textcolor{lightgray}{49.26} & \textcolor{lightgray}{39.04} & \textcolor{lightgray}{33.91} \\ %

                & PanoOcc~\cite{wang2023panoocc} & \textcolor{lightgray}{35.78} & \textcolor{lightgray}{8.18} & \textcolor{lightgray}{41.60} & \textcolor{lightgray}{20.79} & \textcolor{lightgray}{41.25} & \textcolor{lightgray}{47.78} & 21.87 & \textcolor{lightgray}{23.42} & \textcolor{lightgray}{21.03} & \textcolor{lightgray}{19.29} & \textcolor{lightgray}{29.71} & \textcolor{lightgray}{36.10} & 81.20 & \textcolor{lightgray}{40.00} & \textcolor{lightgray}{49.22} & 53.94 & \textcolor{lightgray}{38.09} & \textcolor{lightgray}{34.83}  \\ %

                & PanoOcc$^{\ddagger}$ & 36.63 & 8.64 & \textbf{43.71} & 21.69 & 42.55 & 49.91 & \textcolor{lightgray}{21.32} & \textbf{25.35}
 & \textbf{22.92} & \textbf{20.19} & 29.78 & 37.19 & \textcolor{lightgray}{80.97} & 40.36 & 49.65 & \textcolor{lightgray}{52.84} & 39.81 & 35.82 \\ %

                % & PanoOcc$^{\dag}$ &  36.63 & 8.64 & 43.71 & 21.69 & 42.55 & 49.91 & 21.32 & 25.35 & 22.92 & 20.19 & 29.78 & 37.19 & 80.97 & 40.36 & 49.65 & 52.84 & 39.81 & 35.82  \\ %
                
                & \cellcolor{gray!20}\textbf{ProtoOcc~(Ours)} &  \cellcolor{gray!20}\textbf{37.80} & \cellcolor{gray!20}\textbf{9.28} & \cellcolor{gray!20}43.64 & \cellcolor{gray!20}\textbf{22.30} & \cellcolor{gray!20}\textbf{44.72} & \cellcolor{gray!20}\textbf{50.07} & \cellcolor{gray!20}\textbf{23.68} & \cellcolor{gray!20}25.23 & \cellcolor{gray!20}22.77 & \cellcolor{gray!20}19.66 & \cellcolor{gray!20}\textbf{30.43} & \cellcolor{gray!20}\textbf{38.73} & \cellcolor{gray!20}\textbf{82.05} & \cellcolor{gray!20}\textbf{42.61} & \cellcolor{gray!20}\textbf{51.68} & \cellcolor{gray!20}\textbf{55.84} & \cellcolor{gray!20}\textbf{41.91} &\cellcolor{gray!20}\textbf{38.05} \\ %

			\bottomrule
		\end{tabular}
		}
		\label{tab:app_occ3d}
	\end{table*}

\subsection{Quantitative Results}

\myparagraph{Occ3D-nuScenes.} 
We present an additional comparative result for the $\texttt{Base}$ and $\texttt{Small}$-sized voxel queries. Note that $\dag$ follows the commonly suggested configuration~\cite{li2022bevformer, wang2023panoocc} for $\texttt{Base}$-sized voxel queries with larger image size and more training epochs. 
Furthermore, $\ddag$ indicates that the model utilizes 3D bounding box ground truth. As shown in Table~\ref{tab:app_occ3d}, our method achieves an overall performance improvement across every variant~($\dag$ and $\ddag$), especially surpassing the baselines in several important classes (e.g., cars and pedestrians). 
Notably, compared to $\ddag$, we observe that ProtoOcc exhibits superior performance, despite the absence of explicit geometric and semantic cues derived from the bounding box ground truth of each object. This observation demonstrates that the proposed ProtoOcc method effectively captures visual geometric details from the given RGB images by leveraging high-level image prototypes and multi-perspective decoding strategies regardless of the voxel query sizes.

\myparagraph{SemanticKITTI.} We further present additional qualitative results on the validation and hidden test set with detailed scores over each class. As clearly indicated in Table~\ref{tab:app_sem_kitti_val} and~\ref{tab:app_sem_kitti_test}, we observe that ProtoOcc shows significant improvements across various sizes of voxel query, which is consistent with the previous results in the main manuscript. Specifically, we show that ProtoOcc is also beneficial in test set, indicating the generalizability of our proposed methods.

\myparagraph{Efficiency Comparison.}
The experimental comparisons of the computational efficiencies are reported in table~\ref{tab:vox_cost}. According to the results, due to the reduced voxel size, we notice performance degradations from \texttt{Base} setting to \texttt{Small} setting. However, applying our ProtoOcc on the two baseline~(VoxFormer~\cite{li2023voxformer} and Symphonies~\cite{jiang2024symphonize}) offsets the loss in performances, even outperforming \texttt{Base} performance in mIoU with \texttt{Small} query setting. Note that ProtoOcc achieves this performance with 83.32\%, 54.58\%, and 82.29\% less parameters, inference time and FLOPs, respectively, for VoxFormer. For Symphonies, ProtoOcc saves 53.17\%, 46.46\%, and 67.90\% of parameters, inference time and FLOPs, respectively.

\begin{table}[ht]
    \caption{Comparison of Computational Efficiency.}
    \centering
    \resizebox{\linewidth}{!}{
    \begin{tabular}{llcccc}
            \toprule
            Query Res. & Model &  Inf. Time & FLOPs~(G) & Params & mIoU\\
            \midrule
            \multirow{2}{*}{\parbox{2cm}{$128\times128\times16$ \\ \centering(\texttt{Base})}}
 & VoxFormer-\texttt{B}~\cite{li2023voxformer} &  49.1~ms & 288 & 34.61M & 12.35\\
            & Symphonies-\texttt{B}~\cite{jiang2024symphonize} &  76.2~ms & 162 & 21.59M & 14.38\\\midrule
            \multirow{4}{*}{\parbox{2cm}{$64\times64\times8$ \\ \centering(\texttt{Small})}} & VoxFormer-\texttt{S} &  13.4~ms & 37 & 	5.31M & 11.57\\ 
            & \cellcolor{gray!20}\textbf{+ ProtoOcc--\texttt{S}~(Ours)} &  \cellcolor{gray!20}22.3~ms & \cellcolor{gray!20}51 & \cellcolor{gray!20}5.77M & \cellcolor{gray!20}12.40\\
            & Symphonies-\texttt{S} &  23.5~ms & 46 & 	9.85M & 13.64\\
            & \cellcolor{gray!20}\textbf{+ ProtoOcc--\texttt{S}~(Ours)} &  \cellcolor{gray!20}40.8~ms & \cellcolor{gray!20}52 & \cellcolor{gray!20}10.11M & \cellcolor{gray!20}14.50\\
            \bottomrule
    \end{tabular}}
    % \vspace{-1em}
    \label{tab:vox_cost}
\end{table}

\subsection{Qualitative Results}
\label{app:DB}
In this section, we provide additional qualitative results of 3D occupancy prediction and 3D semantic scene completion.
As clearly shown in Figure~\ref{fig:fig_qual_sup1} and~\ref{fig:fig_qual_sup2}, the high-level 2D semantics enable ProtoOcc to interpret the scene in a more sectionalized manner, producing more detailed predictions over the baseline.
In contrast, the baseline, which does not utilize the explicit guidance of high-level 2D contextual information, confuses the occupied states in empty space~(See $2^{\text{nd}}$ row example of Figure~\ref{fig:fig_qual_sup2}). 
Furthermore, the baseline detects ghost objects, causing serious safety concerns due to misunderstanding the irregular driving surface~(See $1^{\text{st}}$ row example of Figure~\ref{fig:fig_qual_sup1}). 
However, our context-diversified decoding strategy enables precise semantic understanding, by considering the variously augmented context features. Also, from \ref{fig:fig_qual_sem_vox} and \ref{fig:fig_qual_sem_symp}, we observe that applying ProtoOcc can effectively capture the boundaries of the objects in 2D images, which affects depth predictions of the occupancies.

\noindent
\begin{figure}
  \centering
  % \vspace{-1.em}
  \resizebox{\linewidth}{!}{%
      \includegraphics{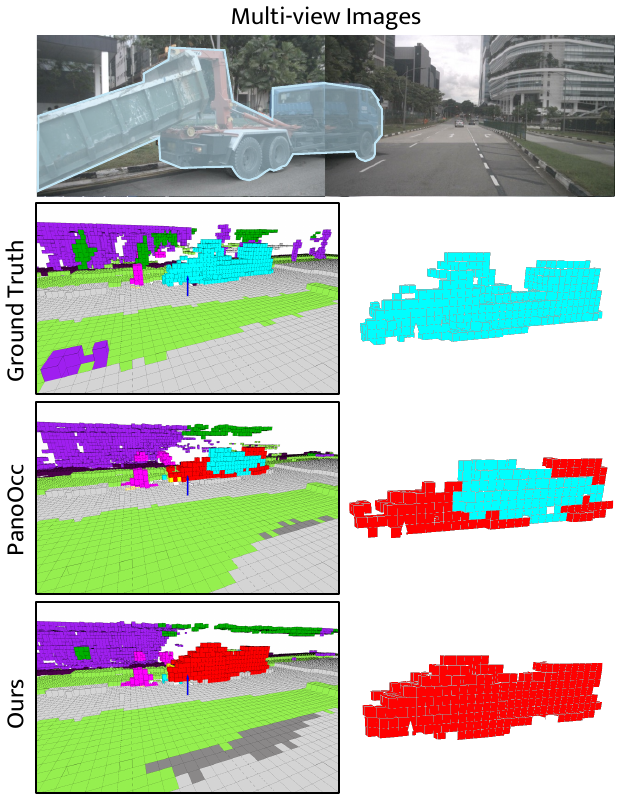}
    }
  \caption{\textbf{Limitation Case.}}
  \label{fig:limit}
\end{figure}

\section{Limitation and Societal Impact}
\label{app:E}
As shown in Figure~\ref{fig:limit}, 
our proposed ProtoOcc misses the class label while accurately predicting the comprehensive geometry of the object.
This phenomenon mainly occurs in the objects with rare classes, which is a long-standing class imbalance problem for the classification tasks. 
Moreover, the prediction of classes bounded in pre-defined labels is unsuitable for the comprehensive understanding of 3D scene.
Thus, we recommend further research to extend the task to an open vocabulary setting, by incorporating the powerful external knowledge of foundation models~(e.g., CLIP~\cite{radford2021learning} and Grounding DINO~\cite{liu2023grounding}). Specifically, our prototype-aware pixel features can be aligned within the text-image embedding space to provide a fine-grained and unbounded understanding of the surrounding scene. We are open to more discussions and suggestions.

\begin{table*}[htb]
    \caption{\textbf{Quantitative results on SemanticKITTI \texttt{val}.} }
    \centering
    \newcommand{\clsname}[2]{
        \rotatebox{90}{
            \hspace{-6pt}
            \textcolor{#2}{$\blacksquare$}
            \hspace{-6pt}
            \renewcommand\arraystretch{0.6}
            \begin{tabular}{l}
                #1                                      \\
                \hspace{-4pt} ~\tiny(\semkitfreq{#2}\%) \\
            \end{tabular}
        }}
    \renewcommand{\tabcolsep}{2pt}
    \renewcommand\arraystretch{1.1}
    \scalebox{0.84}
    {
        \begin{tabular}{l|rr|rrrrrrrrrrrrrrrrrrrr}
            \toprule
            Method                               &
            \multicolumn{1}{c}{IoU}              &
            mIoU                                 &
            \clsname{road}{s_road}                 &
            \clsname{sidewalk}{s_sidewalk}         &
            \clsname{parking}{s_parking}           &
            \clsname{other-grnd.}{s_otherground}   &
            \clsname{building}{s_building}         &
            \clsname{car}{s_car}                   &
            \clsname{truck}{s_truck}               &
            \clsname{bicycle}{s_bicycle}           &
            \clsname{motorcycle}{s_motorcycle}     &
            \clsname{other-veh.}{s_othervehicle}   &
            \clsname{vegetation}{s_vegetation}     &
            \clsname{trunk}{s_trunk}               &
            \clsname{terrain}{s_terrain}           &
            \clsname{person}{s_person}             &
            \clsname{bicyclist}{s_bicyclist}       &
            \clsname{motorcyclist}{s_motorcyclist} &
            \clsname{fence}{s_fence}               &
            \clsname{pole}{s_pole}                 &
            \clsname{traf.-sign}{s_trafficsign}
            \\
            \midrule
            LMSCNet~\cite{roldao2020lmscnet} & 28.61 & 6.70  & 40.68 & 18.22 & 4.38  & 0.00  & 10.31 & 18.33 & 0.00  & 0.00 & 0.00 & 0.00  & 13.66 & 0.02  & 20.54 & 0.00 & 0.00 & 0.00 & 1.21 & 0.00 & 0.00 \\
            AICNet~\cite{li2020anisotropic} & 29.59 & 8.31  & 43.55 & 20.55 & 11.97 & 0.07  & 12.94 & 14.71 & 4.53  & 0.00 & 0.00 & 0.00  & 15.37 & 2.90  & 28.71 & 0.00 & 0.00 & 0.00 & 2.52 & 0.06 & 0.00 \\
            JS3C-Net~\cite{yan2021sparse} & 38.98 & 10.31 & 50.49 & 23.74 & 11.94 & 0.07 & 15.03& 24.65& 4.41 & 0.00& 0.00& 6.15 & 18.11& 4.33 & 26.86& 0.67& 0.27& 0.20 & 3.94& 3.77& 1.45\\
            MonoScene~\cite{cao2022monoscene}    & 36.86& 11.08& 56.52& 26.72& 14.27& 0.46 & 14.09& 23.26& 6.98 & 0.61& 0.45& 1.48 & 17.89& 2.81 & 29.64& 1.86& 1.20& 0.00& 5.84& 4.14& 2.25\\
            TPVFormer~\cite{huang2023tri} & 35.61& 11.36& 56.50& 25.87& 20.60& 0.85 & 13.88& 23.81& 8.08 & 0.36& 0.05& 4.35 & 16.92& 2.26 & 30.38& 0.51& 0.89& 0.00& 5.94& 3.14& 1.52\\
            OccFormer~\cite{zhang2023occformer} & 36.50& 13.46& 58.85& 26.88& 19.61& 0.31 & 14.40& 25.09& 25.53 & 0.81& 1.19& 8.52 & 19.63& 3.93 & 32.62 & 2.78& 2.82& 0.00& 5.61& 4.26& 2.86\\
            HASSC~\cite{wang2024not}  & 44.82 & 13.48 & 57.05 & 28.25 & 15.90 & 1.04 & 19.05 & 27.23 & 9.91 & 0.92 & 0.86 & 5.61 & 25.48 & 6.15 & 32.94 & 2.80 & 4.71 & 0.00 & 6.58 & 7.68 & 4.05 \\
            \hline
            
            VoxFormer-\texttt{S}~\cite{li2023voxformer}  & 43.10 & 11.51 & 53.71 & 26.04 & 13.18 & 0.09 & 18.91 & 24.39 & 1.80 & 1.14 & 0.13 & 1.46 & 25.22 & 5.71 & 31.93 & 0.67 & 1.14 & 0.00 & 5.80 & 5.51 & 2.75 \\
            
            \cellcolor{gray!20}+ ProtoOcc~(Ours)  & \cellcolor{gray!20}43.55 & \cellcolor{gray!20}12.39 & \cellcolor{gray!20}56.06 & \cellcolor{gray!20}26.96 & \cellcolor{gray!20}13.28 & \cellcolor{gray!20}0.29  & \cellcolor{gray!20}19.00 & \cellcolor{gray!20}24.69 & \cellcolor{gray!20}9.85 & \cellcolor{gray!20}0.18 & \cellcolor{gray!20}0.23 & \cellcolor{gray!20}3.23 & \cellcolor{gray!20}25.74 & \cellcolor{gray!20}5.57  & \cellcolor{gray!20}33.89 & \cellcolor{gray!20}1.03 & \cellcolor{gray!20}1.14 & \cellcolor{gray!20}0.00 & \cellcolor{gray!20}6.32 & \cellcolor{gray!20}5.33 & \cellcolor{gray!20}2.65 \\
            
            VoxFormer-\texttt{B}~\cite{li2023voxformer} & 44.02 & 12.35& 54.76& 26.35& 15.50& 0.70 & 17.65& 25.79& 5.63 & 0.59& 0.51& 3.77 & 24.39& 5.08 & 29.96& 1.78& 3.32 & 0.00& 7.64& 7.11& 4.18\\
            
            \cellcolor{gray!20}+ ProtoOcc~(Ours)  & \cellcolor{gray!20}\textbf{44.90} & \cellcolor{gray!20}13.57 & \cellcolor{gray!20}58.11 & \cellcolor{gray!20}28.83 & \cellcolor{gray!20}17.52 & \cellcolor{gray!20}0.54 & \cellcolor{gray!20}19.72 & \cellcolor{gray!20}27.43 & \cellcolor{gray!20}12.14 & \cellcolor{gray!20}0.24 & \cellcolor{gray!20}0.16 & \cellcolor{gray!20}3.21 & \cellcolor{gray!20}26.42 & \cellcolor{gray!20}6.54 & \cellcolor{gray!20}34.31 & \cellcolor{gray!20}1.26 & \cellcolor{gray!20}2.89 & \cellcolor{gray!20}0.00 & \cellcolor{gray!20}7.87 & \cellcolor{gray!20}7.43 & \cellcolor{gray!20}3.31 \\
            \hline
            Symphonies-\texttt{S}~\cite{jiang2024symphonize}  & 41.67 & 13.64 & 56.86 & 27.73 & 18.23 & 0.33 & 21.37 & 26.24 & 9.23 & 1.98 & 0.71 & 8.16 & 24.47 & 5.87 & 30.68 & 3.29 & 3.32 & 0.00 & 7.27 & 8.03 & 5.32 \\
            \cellcolor{gray!20}+ ProtoOcc~(Ours)  & \cellcolor{gray!20}43.02 & \cellcolor{gray!20}14.50 & \cellcolor{gray!20}57.84 & \cellcolor{gray!20}28.27 & \cellcolor{gray!20}17.94 & \cellcolor{gray!20}0.09  & \cellcolor{gray!20}22.81 & \cellcolor{gray!20}27.67 & \cellcolor{gray!20}15.96 & \cellcolor{gray!20}1.69 & \cellcolor{gray!20}1.63 & \cellcolor{gray!20}11.46 & \cellcolor{gray!20}26.13 & \cellcolor{gray!20}5.29  & \cellcolor{gray!20}32.48 & \cellcolor{gray!20}3.22 & \cellcolor{gray!20}2.54 & \cellcolor{gray!20}0.00 & \cellcolor{gray!20}7.70 & \cellcolor{gray!20}7.54 & \cellcolor{gray!20}5.23 \\
            Symphonies-\texttt{B}~\cite{jiang2024symphonize}& 41.85& 14.38 & 56.52& 26.29& 18.08 & 0.02 & 22.22 & 29.19 & 10.75& 2.86 & 2.87 & 10.60 & 25.62 & 6.53 & 30.29 & 3.92 & 3.13& 0.00& 8.12 & 9.85 & 6.09 \\
            \cellcolor{gray!20}+ ProtoOcc~(Ours)  & \cellcolor{gray!20}42.12 & \cellcolor{gray!20}\textbf{14.83} & \cellcolor{gray!20}56.95 & \cellcolor{gray!20}27.46 & \cellcolor{gray!20}18.29 & \cellcolor{gray!20}0.02  & \cellcolor{gray!20}22.07 & \cellcolor{gray!20}29.32 & \cellcolor{gray!20}14.46 & \cellcolor{gray!20}3.24 & \cellcolor{gray!20}2.54 & \cellcolor{gray!20}13.66 & \cellcolor{gray!20}25.87 & \cellcolor{gray!20}6.19  & \cellcolor{gray!20}30.76 & \cellcolor{gray!20}3.79 & \cellcolor{gray!20}3.11 & \cellcolor{gray!20}0.00 & \cellcolor{gray!20}8.93 & \cellcolor{gray!20}9.20 & \cellcolor{gray!20}5.76 \\
            \bottomrule
        \end{tabular}
    }
    \label{tab:app_sem_kitti_val}
\end{table*}

\begin{table*}[ht]
    \caption{\textbf{Quantitative results on SemanticKITTI \texttt{test}.}}
    \centering
    \newcommand{\clsname}[2]{
        \rotatebox{90}{
            \hspace{-6pt}
            \textcolor{#2}{$\blacksquare$}
            \hspace{-6pt}
            \renewcommand\arraystretch{0.6}
            \begin{tabular}{l}
                #1                                      \\
                \hspace{-4pt} ~\tiny(\semkitfreq{#2}\%) \\
            \end{tabular}
        }}
    \renewcommand{\tabcolsep}{2pt}
    \renewcommand\arraystretch{1.1}
    \scalebox{0.84}
    {
        \begin{tabular}{l|rr|rrrrrrrrrrrrrrrrrrrr}
            \toprule
            Method                               &
            \multicolumn{1}{c}{IoU}              &
            mIoU                                 &
            \clsname{road}{s_road}                 &
            \clsname{sidewalk}{s_sidewalk}         &
            \clsname{parking}{s_parking}           &
            \clsname{other-grnd.}{s_otherground}   &
            \clsname{building}{s_building}         &
            \clsname{car}{s_car}                   &
            \clsname{truck}{s_truck}               &
            \clsname{bicycle}{s_bicycle}           &
            \clsname{motorcycle}{s_motorcycle}     &
            \clsname{other-veh.}{s_othervehicle}   &
            \clsname{vegetation}{s_vegetation}     &
            \clsname{trunk}{s_trunk}               &
            \clsname{terrain}{s_terrain}           &
            \clsname{person}{s_person}             &
            \clsname{bicyclist}{s_bicyclist}       &
            \clsname{motorcyclist}{s_motorcyclist} &
            \clsname{fence}{s_fence}               &
            \clsname{pole}{s_pole}                 &
            \clsname{traf.-sign}{s_trafficsign}
            \\
            \midrule
            LMSCNet~\cite{roldao2020lmscnet}     & 31.38 & 7.07  & 46.70 & 19.50 & 13.50 & 3.10  & 10.30 & 14.30 & 0.30 & 0.00 & 0.00 & 0.00 & 10.80 & 0.00  & 10.40 & 0.00 & 0.00 & 0.00 & 5.40  & 0.00 & 0.00 \\
            AICNet~\cite{li2020anisotropic}       & 23.93 & 7.09  & 39.30 & 18.30 & 19.80 & 1.60  & 9.60  & 15.30 & 0.70 & 0.00 & 0.00 & 0.00 & 9.60  & 1.90  & 13.50 & 0.00 & 0.00 & 0.00 & 5.00  & 0.10 & 0.00 \\
            JS3C-Net~\cite{yan2021sparse}    & 34.00 & 8.97  & 47.30 & 21.70 & 19.90 & 2.80  & 12.70 & 20.10 & 0.80 & 0.00 & 0.00 & 4.10 & 14.20 & 3.10  & 12.40 & 0.00 & 0.20 & 0.20 & 8.70  & 1.90 & 0.30 \\
            MonoScene~\cite{cao2022monoscene}    & 34.16 & 11.08 & 54.70 & 27.10 & 24.80 & 5.70  & 14.40 & 18.80 & 3.30 & 0.50 & 0.70 & 4.40 & 14.90 & 2.40  & 19.50 & 1.00 & 1.40 & 0.40 & 11.10 & 3.30 & 2.10 \\
            TPVFormer~\cite{huang2023tri}  & 34.25 & 11.26 & 55.10 & 27.20 & 27.40 & 6.50  & 14.80 & 19.20 & 3.70 & 1.00 & 0.50 & 2.30 & 13.90 & 2.60  & 20.40 & 1.10 & 2.40 & 0.30 & 11.00 & 2.90 & 
            1.50 \\
            OccFormer~\cite{zhang2023occformer}  & 34.53 & 12.32 & 55.90 & 30.30 & 31.50 & 6.50  & 15.70 & 21.60 & 1.20 & 1.50 & 1.70 & 3.20 & 16.80 & 3.90  & 21.30 & 2.20 & 1.10 & 0.20 & 11.90 & 3.80 & 3.70 \\
            HASSC~\cite{wang2024not}  & 43.40 & 13.34 & 54.60 & 27.70 & 23.80 & 6.20 & 21.10 & 22.80 & 4.70 & 1.60 & 1.00 & 3.90 & 23.80 & 8.50 & 23.30 & 1.60 & 4.00 & 0.30 & 13.01 & 5.80 & 5.50 \\
            \hline
            VoxFormer-\texttt{S}~\cite{li2023voxformer}  & 42.56 & 11.28 & 51.30 & 24.80 & 18.50 & 2.70 & 21.40 & 19.7 & 1.00 & 0.40 & 0.20 & 1.10 & 24.70 & 5.90 & 21.10 & 0.70 & 0.60 & 0.20 & 11.60 & 4.00 & 4.30 \\
            \cellcolor{gray!20}+ ProtoOcc~(Ours)  & \cellcolor{gray!20}42.20 & \cellcolor{gray!20}11.60 & \cellcolor{gray!20}54.50 & \cellcolor{gray!20}26.30 & \cellcolor{gray!20}19.40 & \cellcolor{gray!20}3.90  & \cellcolor{gray!20}20.80 & \cellcolor{gray!20}19.80 & \cellcolor{gray!20}1.70 & \cellcolor{gray!20}0.80 & \cellcolor{gray!20}0.30 & \cellcolor{gray!20}1.80 & \cellcolor{gray!20}23.80 & \cellcolor{gray!20}6.20  & \cellcolor{gray!20}21.30 & \cellcolor{gray!20}0.70 & \cellcolor{gray!20}0.50 & \cellcolor{gray!20}0.10 & \cellcolor{gray!20}10.20 & \cellcolor{gray!20}4.00 & \cellcolor{gray!20}4.30 \\
            VoxFormer-\texttt{B}~\cite{li2023voxformer}  & 42.95 & 12.20 & 53.90 & 25.30 & 21.10 & 5.60  & 19.80 & 20.80 & 3.50 & 1.00 & 0.70 & 3.70 & 22.40 & 7.50  & 21.30 & 1.40 & 2.60 & 0.20 & 11.10 & 5.10 & 4.90 \\
            \cellcolor{gray!20}+ ProtoOcc~(Ours)  & \cellcolor{gray!20}\textbf{43.87} & \cellcolor{gray!20}12.81 & \cellcolor{gray!20}57.10 & \cellcolor{gray!20}28.20 & \cellcolor{gray!20}22.80 & \cellcolor{gray!20}4.30  & \cellcolor{gray!20}21.70 & \cellcolor{gray!20}22.40 & \cellcolor{gray!20}2.70 & \cellcolor{gray!20}0.80 & \cellcolor{gray!20}0.40 & \cellcolor{gray!20}1.60 & \cellcolor{gray!20}24.90 & \cellcolor{gray!20}7.90  & \cellcolor{gray!20}22.60 & \cellcolor{gray!20}0.90 & \cellcolor{gray!20}0.90 & \cellcolor{gray!20}0.30 & \cellcolor{gray!20}12.30 & \cellcolor{gray!20}5.80 & \cellcolor{gray!20}5.70 \\

            \hline
            Symphonies-\texttt{S}~\cite{jiang2024symphonize}  & 42.04 & 14.07 & 57.60 & 29.40 & 29.00 & 10.50 & 24.20 & 22.00 & 2.70 & 2.00 & 1.80 & 4.70 & 23.80 & 7.50 & 22.80 & 2.10 & 1.40 & 0.70 & 13.80 & 5.60 & 5.70 \\
            \cellcolor{gray!20}+ ProtoOcc~(Ours)  & \cellcolor{gray!20}42.21 & \cellcolor{gray!20}14.36 & \cellcolor{gray!20}57.20 & \cellcolor{gray!20}30.40 & \cellcolor{gray!20}30.00 & \cellcolor{gray!20}10.10  & \cellcolor{gray!20}24.50 & \cellcolor{gray!20}22.30 & \cellcolor{gray!20}2.80 & \cellcolor{gray!20}2.00 & \cellcolor{gray!20}1.70 & \cellcolor{gray!20}4.30 & \cellcolor{gray!20}24.50 & \cellcolor{gray!20}8.10  & \cellcolor{gray!20}23.20 & \cellcolor{gray!20}2.30 & \cellcolor{gray!20}2.20 & \cellcolor{gray!20}0.40 & \cellcolor{gray!20}14.60 & \cellcolor{gray!20}6.20 & \cellcolor{gray!20}6.30 \\
            Symphonies-\texttt{B}~\cite{jiang2024symphonize} & 41.82 & 14.50 & 57.00 & 28.00 & 27.50 & 9.10 & 24.10 & 23.70 & 3.70 & 3.60 & 2.40 & 4.40 & 24.60 & 9.90 & 22.50 & 2.90 & 1.70 & 0.50 & 15.70 & 7.50 & 7.00 \\
            \cellcolor{gray!20}+ ProtoOcc~(Ours)  & \cellcolor{gray!20}42.17 & \cellcolor{gray!20}\textbf{14.77} & \cellcolor{gray!20}57.90 & \cellcolor{gray!20}28.60 & \cellcolor{gray!20}27.60 & \cellcolor{gray!20}10.20  & \cellcolor{gray!20}24.30 & \cellcolor{gray!20}24.10 & \cellcolor{gray!20}3.10 & \cellcolor{gray!20}3.30 & \cellcolor{gray!20}3.20 & \cellcolor{gray!20}4.70 & \cellcolor{gray!20}25.00 & \cellcolor{gray!20}9.20  & \cellcolor{gray!20}22.60 & \cellcolor{gray!20}3.40 & \cellcolor{gray!20}2.00 & \cellcolor{gray!20}1.50 & \cellcolor{gray!20}15.60 & \cellcolor{gray!20}7.30 & \cellcolor{gray!20}6.90 \\
            \bottomrule
        \end{tabular}
    }
    \label{tab:app_sem_kitti_test}
\end{table*}

\begin{figure*}[h!]
\begin{center}
   \includegraphics[width=0.9\linewidth]{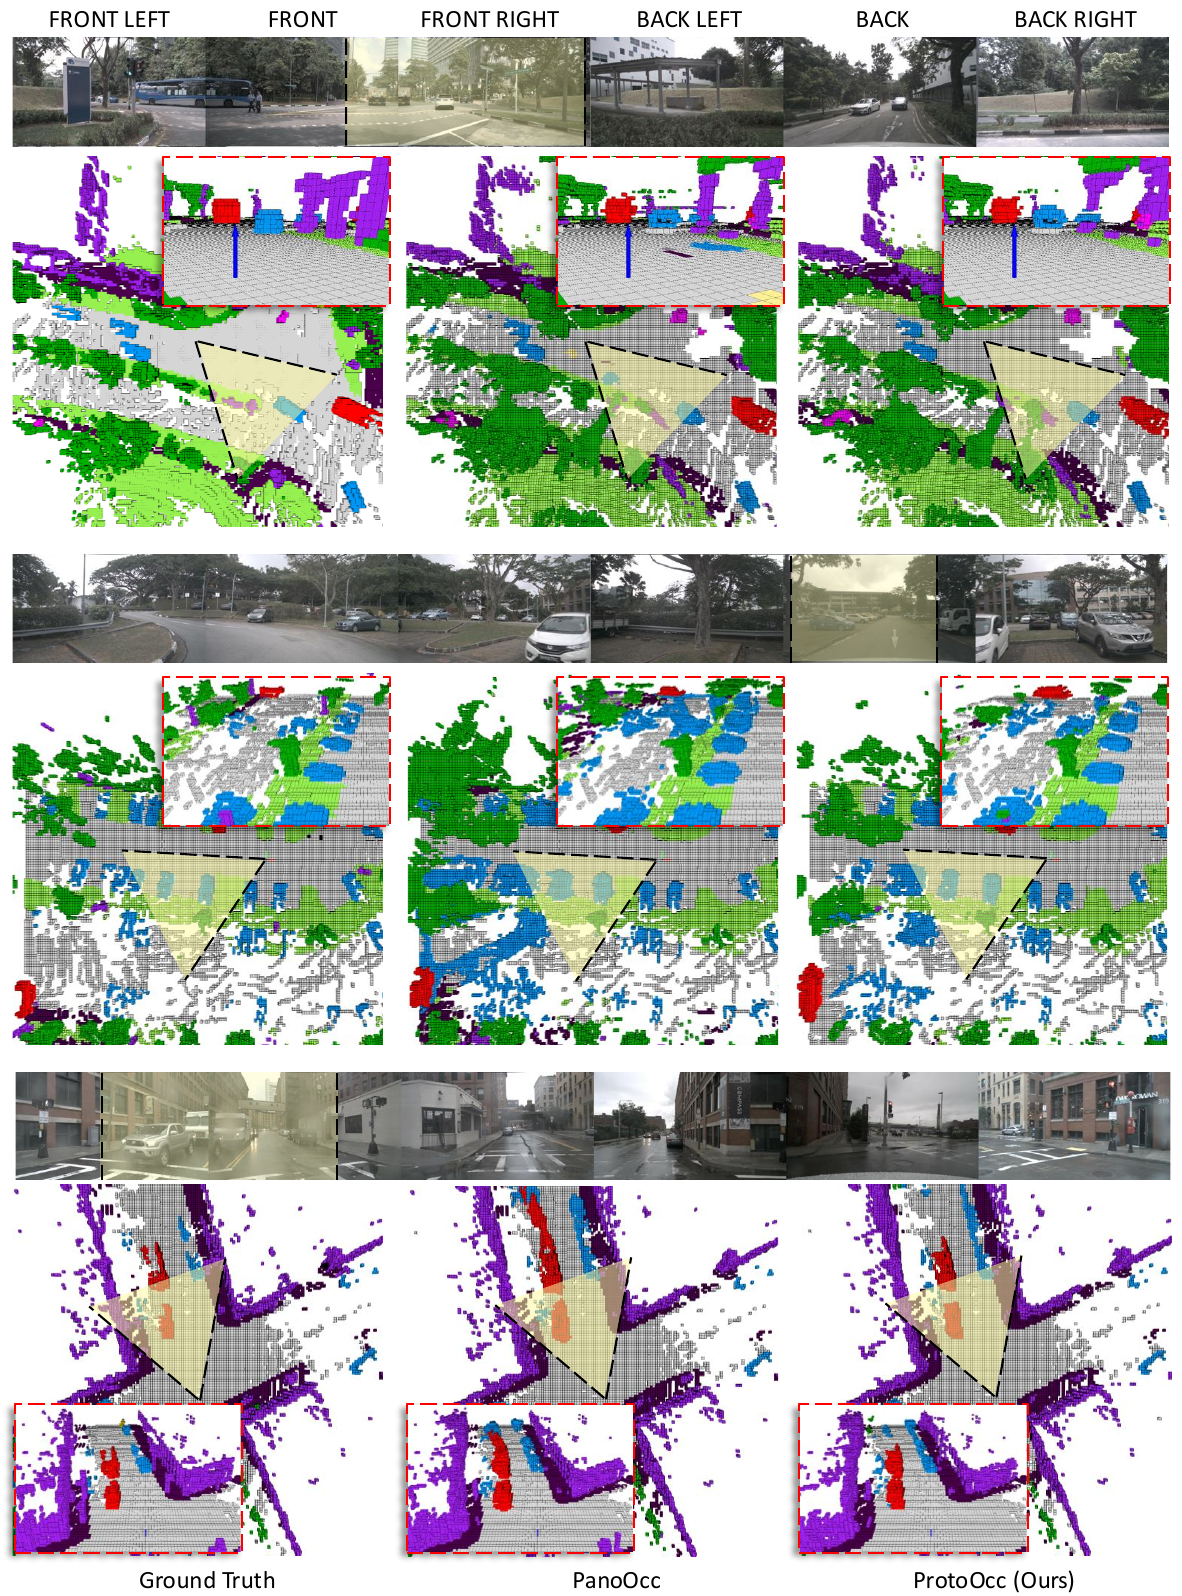}
\end{center}
\vspace{-1.0em}
\caption{\textbf{Predictions in challenging scenarios.} We visualize the prediction results in both aerial and zoomed views, where the zoomed view point is highlighted in yellow. Best viewed in color.}
\label{fig:fig_qual_sup1}
\end{figure*}

\begin{figure*}[h!]
\begin{center}
   \includegraphics[width=0.9\linewidth]{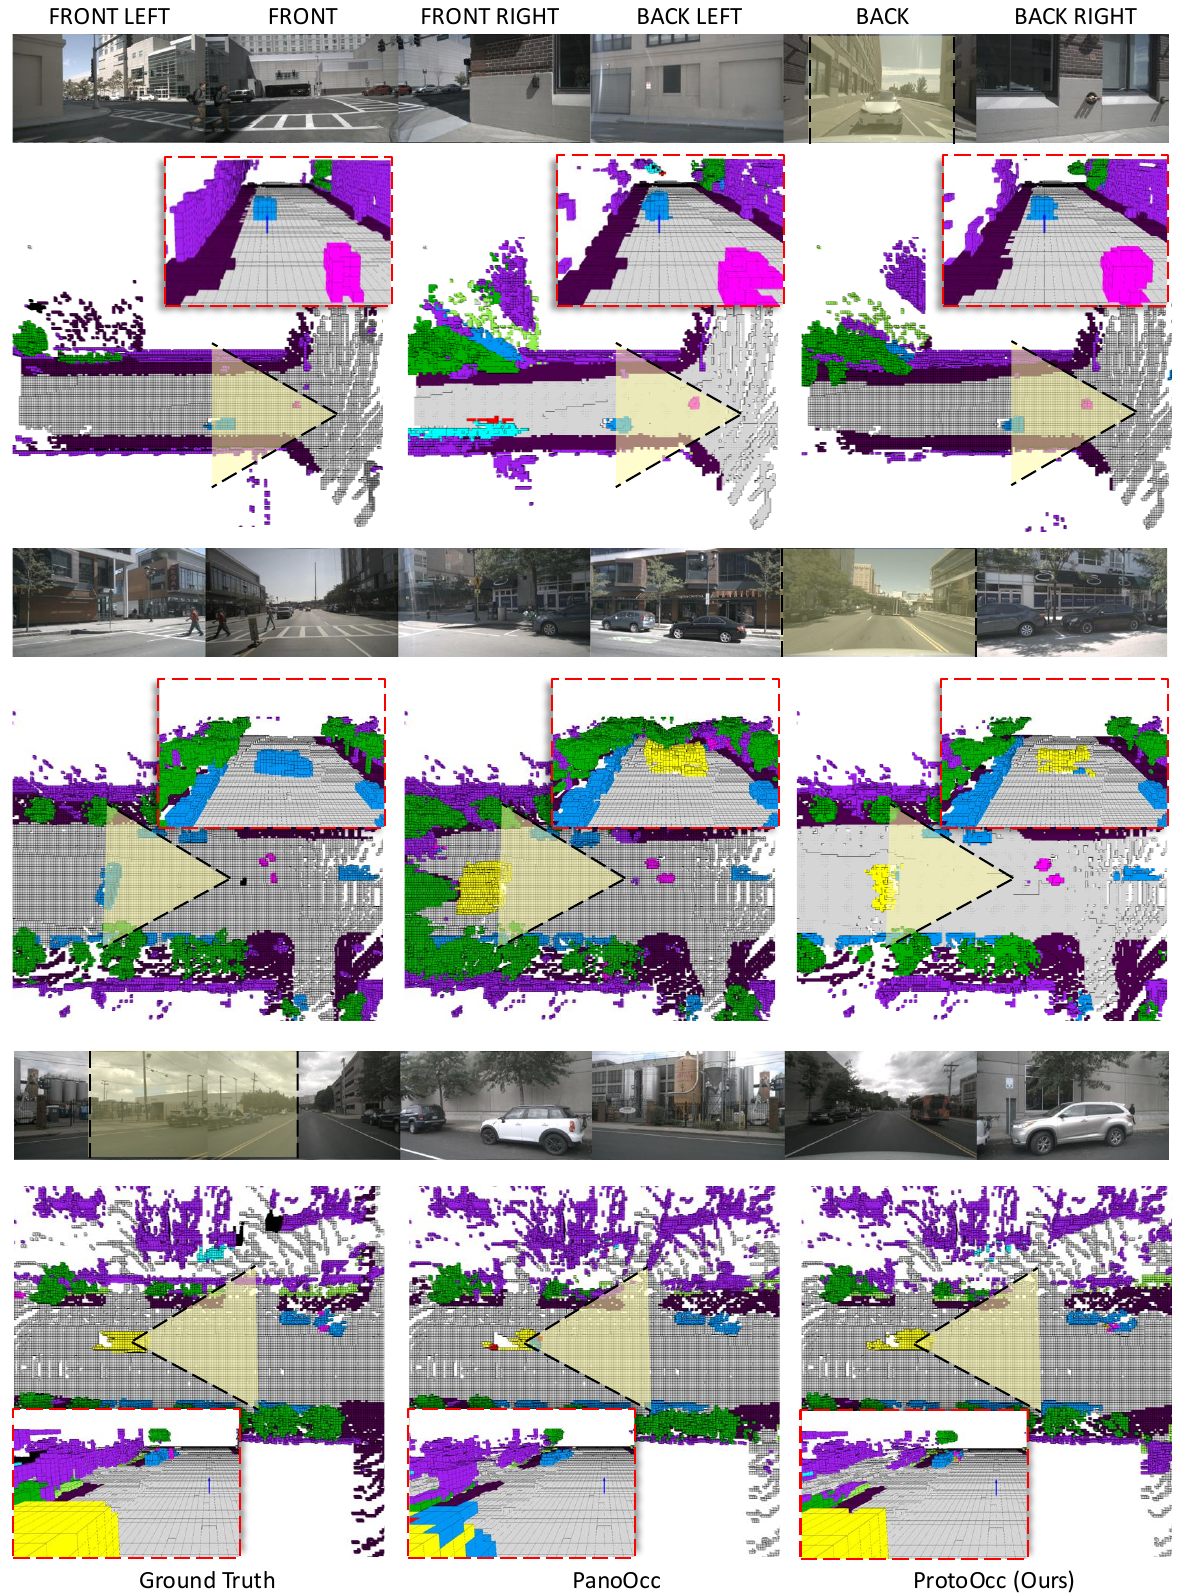}
\end{center}
\vspace{-1.0em}
\caption{\textbf{Predictions in challenging scenarios.} We visualize the prediction results in both aerial and zoomed views, where the zoomed view point is highlighted in yellow. Best viewed in color.}
\label{fig:fig_qual_sup2}
\end{figure*}

\begin{figure*}[t]
\begin{center}
\includegraphics[width=\linewidth]{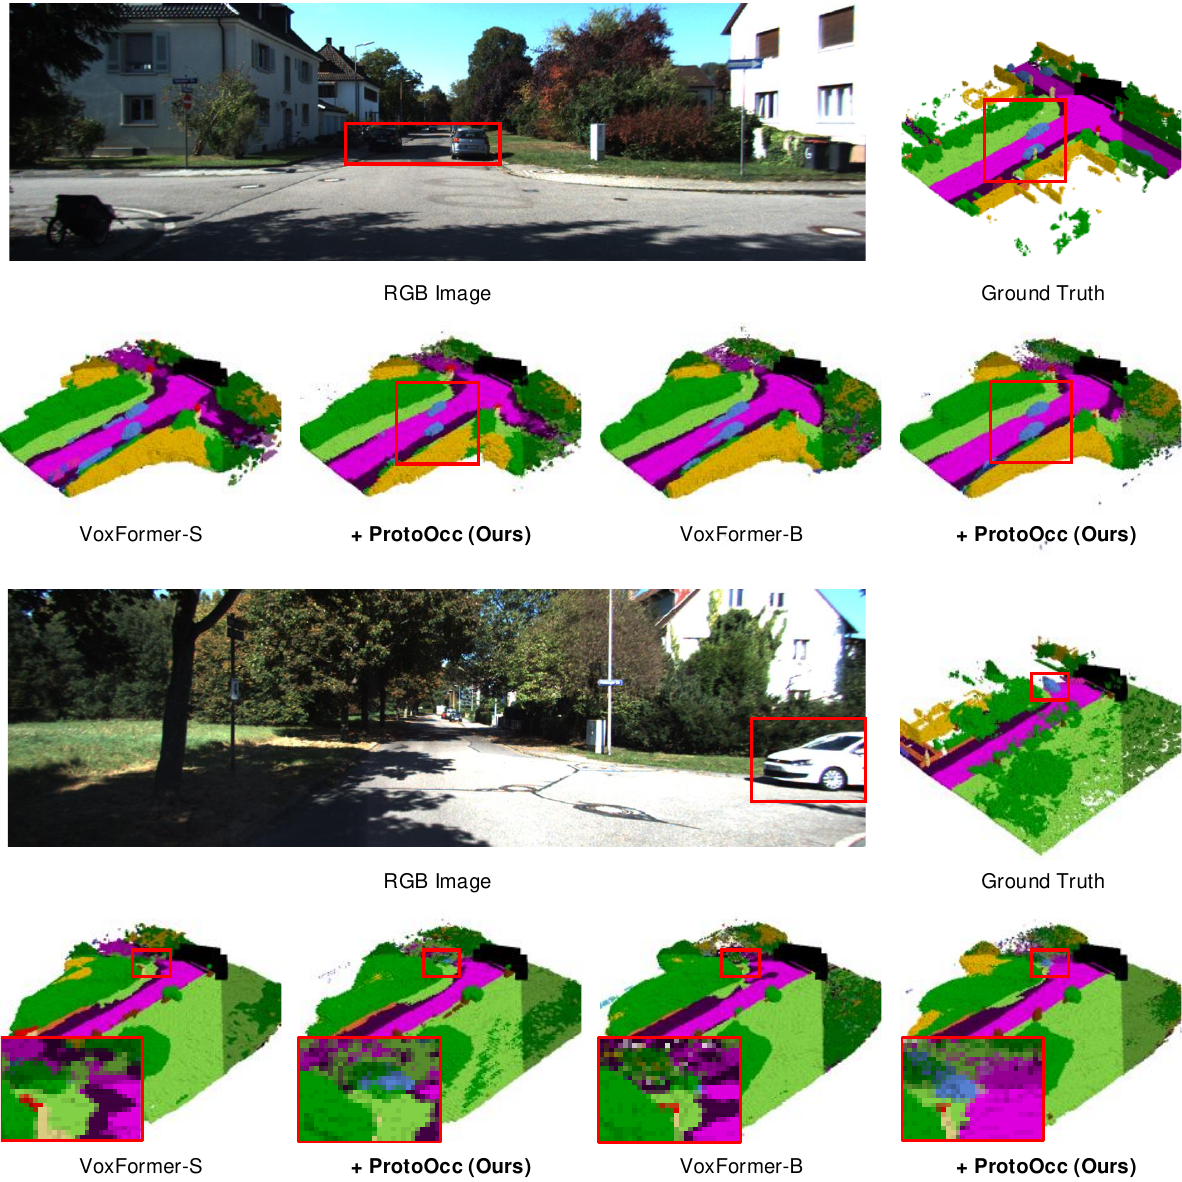}
\end{center}
\vspace{-1.5em}
\caption{\textbf{Qualitative results on SemanticKITTI.}}
\label{fig:fig_qual_sem_vox}
\end{figure*}

\begin{figure*}[t]
\begin{center}
\includegraphics[width=\linewidth]{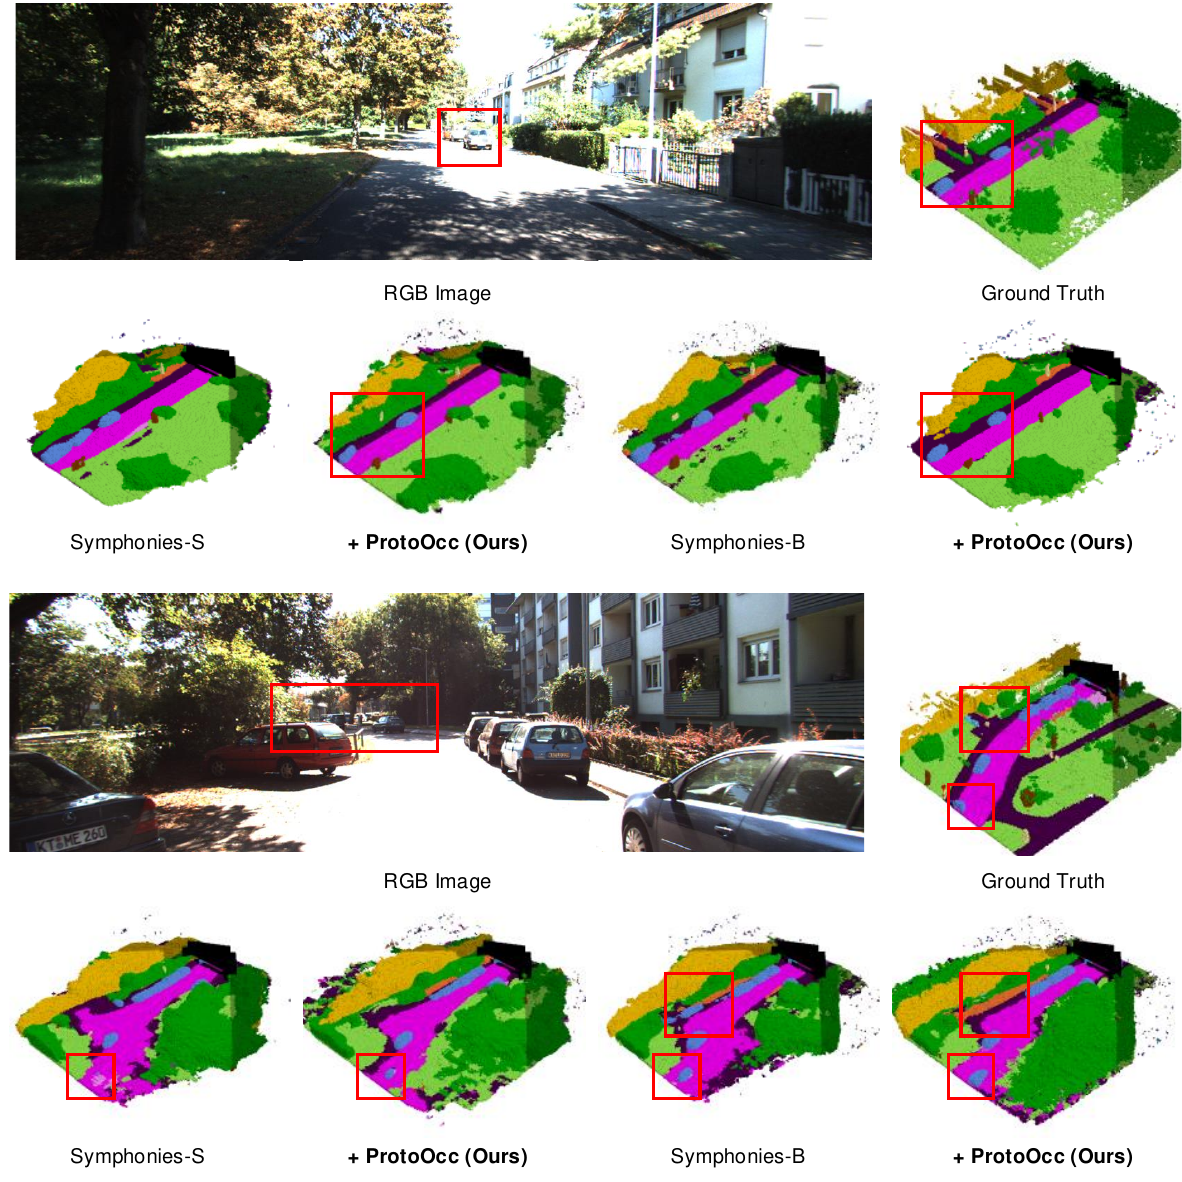}
\end{center}
\vspace{-1.5em}
\caption{\textbf{Qualitative results on SemanticKITTI.}}
\label{fig:fig_qual_sem_symp}
\end{figure*}
